# Supplementary material for: A Mini-Block Fisher Method for Deep Neural Networks
Source: arXiv:2202.04124 source file (2022-10-26)
Supplement: Supplementary file 1 [file implementation.tex]

\subsection{Specification on Algorithms}
\label{sec_10}

% \ref{sec_9}
% \ref{sec_10} no

\begin{algorithm}
    \caption{KFAC}
    \label{algo_1}
    \begin{algorithmic}[1]

    \REQUIRE Given learning rate
    $\alpha$, damping value $\lambda$, batch size $m$, inversion frequency $T$
    
    % \STATE \clarify{how to initialize $A$ and $G$}

    \STATE $\widehat{\mathcal{D} W_l} = 0$, $\Omega_l = \mathbb{E}_n \left[ \sum_{t \in \mathcal{T}} \va_t^{l}(n) \va_t^{l}(n)^\top \right]$, $\Gamma_l = \mathbb{E}_n \left[ \overline{\mathcal{D} \vh^{l}(n) (\mathcal{D} \vh^{l} (n))^\top} \right]$ ($l = 1, ..., L$)
    \COMMENT{Initialization}

    \FOR {$k=1,2,\ldots$}
        \STATE Sample mini-batch $M_k$ of size $m$
        
        \STATE Perform a forward-backward pass over the current mini-batch $M_k$ to compute $\widetilde{\mathcal{D} W_l}$ for $l = 1, ..., L$
        
        \FOR {$l=1,2,\ldots L$}
            
            \STATE $\widehat{\mathcal{D} W_l} = \beta \widehat{\mathcal{D} W_l} + (1-\beta) \widetilde{\mathcal{D} W_l}$
            
            \STATE
            {$p_l = H_{\Gamma}^{l} \widehat{\mathcal{D} W_l} H_{\Omega}^l$}
            \label{line_5}

            \STATE 
            {$W_l = W_l - \alpha \cdot p_{l}$}.
        \ENDFOR
        
        \STATE Perform another pass over $M_k$ with $y$ sampled from the predictive distribution to compute $\mathcal{D} \vh_t^l$ for $l = 1, ..., L$
        % \label{line_2}
        
        \FOR {$l=1,2,\ldots L$}
        
        \STATE Update
        % \deletethis{$\Omega_l = \beta \cdot \Omega_l + (1-\beta) \cdot \overline{\va_{l-1} \va_{l-1}^\top}$}
        {$\Omega_l = \beta \cdot \Omega_l + (1-\beta) \cdot \widetilde{\sum_{t \in \mathcal{T}} \va_t^{l} (\va_t^{l})^\top}$},
        $\Gamma_l = \beta \cdot \Gamma_l + (1-\beta) \cdot \widetilde{\overline{\mathcal{D} \vh_t^{l} (\mathcal{D} \vh_t^{l})^\top}}$
        \label{line_3}
        
        \IF {$i \equiv 0 \pmod{T}$}
            
            \STATE 
            Recompute
            % \deletethis{$H_a^l = (\Omega_l + \sqrt{\lambda} I)^{-1}$}
            {$H_{\Omega}^l = (\Omega_l + \sqrt{\lambda} I)^{-1}$},
            % \deletethis{$H_g^l = (\Gamma_l + \sqrt{\lambda} I)^{-1}$}
            $H_{\Gamma}^l = (\Gamma_l + \sqrt{\lambda} I)^{-1}$
            \label{line_4}
        
        \ENDIF
        
        \ENDFOR

        \ENDFOR  
    
    \end{algorithmic}
\end{algorithm}

We describe the version of KFAC that we implemented in Algorithm \ref{algo_1}. 
Note that $\Omega_l$ in KFAC is the same as $A_l$ is our paper. 
Similar to the pseudo-code of KF-QN-CNN, we assume that all layers are convolutional.

{
Note that KFC-pre in \cite{grosse2016kronecker} differs from Algorithm \ref{algo_1} in the following ways:
\begin{itemize}
    
    \item KFC-pre uses $\pi_l$ to decide how to split $\lambda$ into $\lambda_\Omega$ and $\lambda_\Gamma$
    
    \item KFC-pre uses clipping for the approximated natural gradient direction $p$
    
    % \item momentum on $p$
    
    \item KFC-pre uses momentum for $p$
    
    \item KFC-pre
    uses parameter averaging on $\theta$

\end{itemize}
Note that most of these techniques can also be applied to KF-QN-CNN. Since we are primarily interested in comparing different pre-conditioning matrices, we chose not to include such techniques in our implementation.

}

Also note that in Algorithm \ref{algo_1}, a warm start computation of $\Omega_l$ and $\Gamma_l$ is included, i.e. initial estimates of $\Omega_l$ and $\Gamma_l$ are computed from the whole dataset before the first iteration. A similar warm start computation of $A_l$ was also included in KF-QN-CNN. Since these warm start computations take no more than the time for one epoch, we did not include the times for warm starts in the figures.

% \clarify{describe SGD-m and Adam}

Finally, Adam was implemented exactly as in \cite{kingma2014adam}.
